# Supplementary material for: MOOSE ProbML: Parallelized Probabilistic Machine Learning and Uncertainty Quantification for Computational Energy Applications
Source: arXiv:2504.17101 source file (2025-04-23)
Supplement: Supplementary file 1 [file Appendix.tex]

\begin{figure}[htb!]
    \centering
    \begin{subfigure}[b]{0.49\textwidth} \centering
        \includegraphics[width=\linewidth]{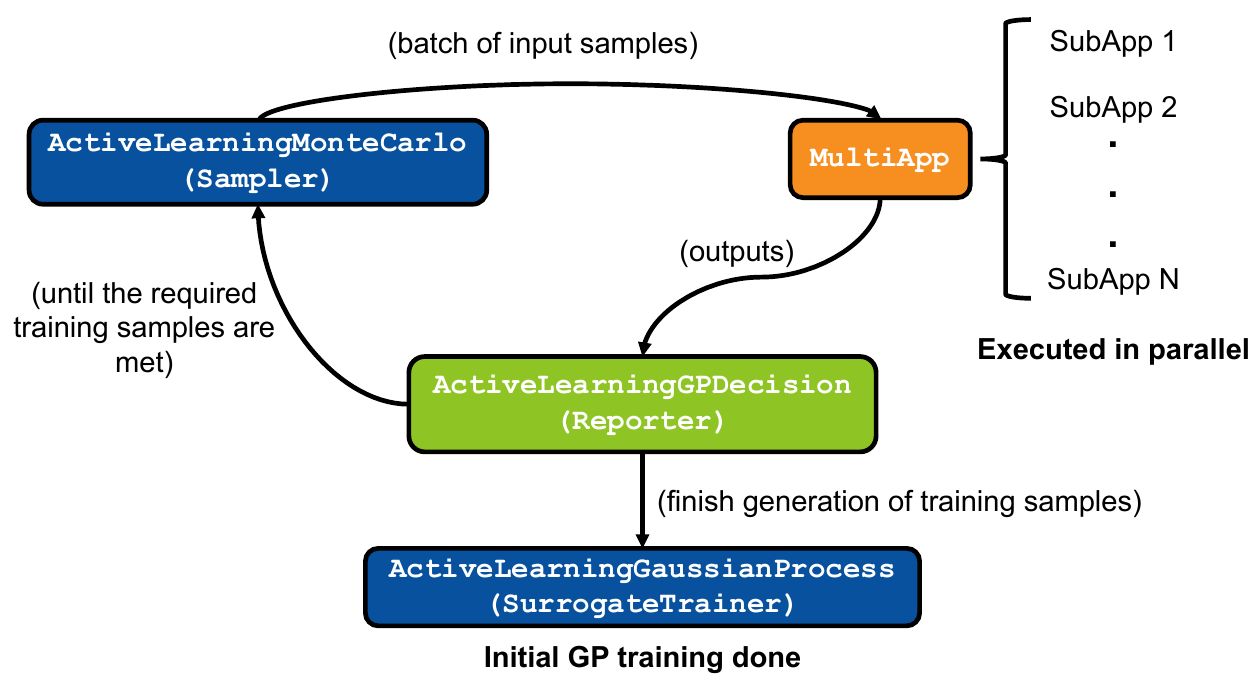}
        \caption{}
        \label{fig:al_train}
    \end{subfigure}
    \hfill
    \begin{subfigure}[b]{0.49\textwidth} \centering
        \includegraphics[width=\linewidth]{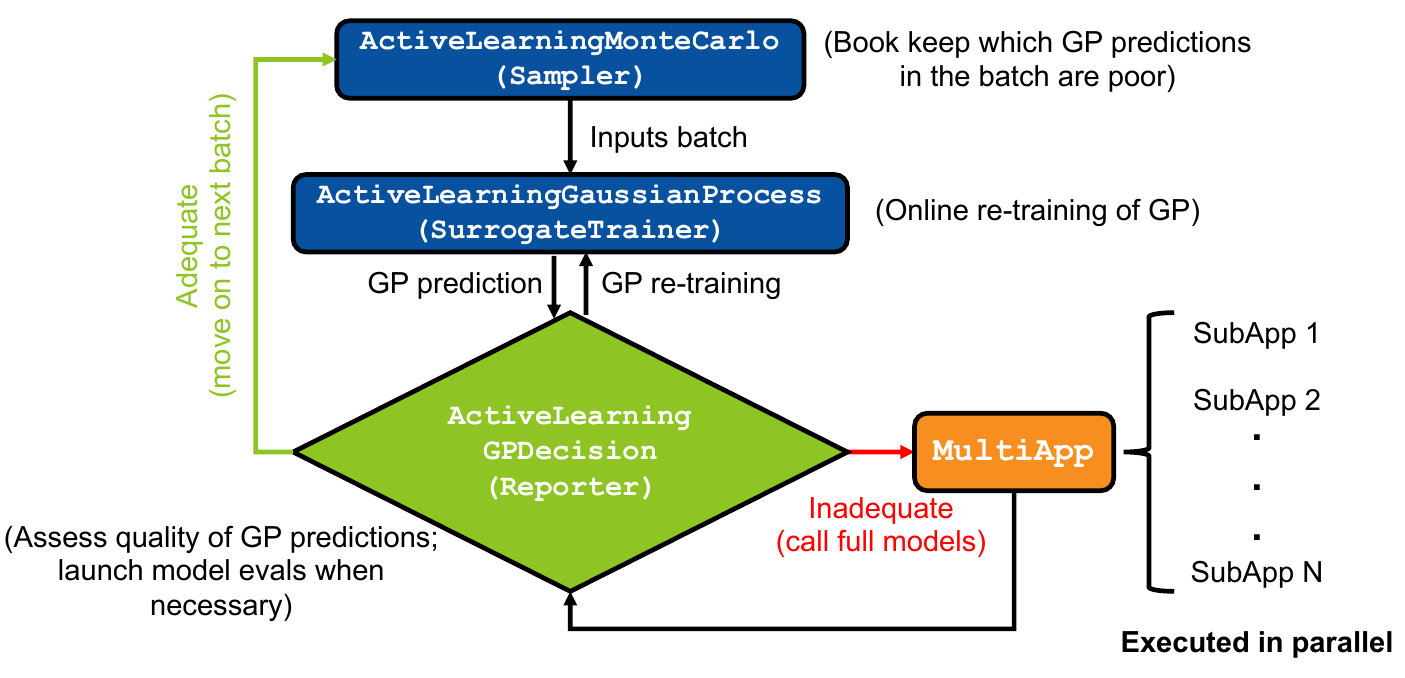}
        \caption{}
        \label{fig:al_eval}
    \end{subfigure}
    \caption{}
    \label{fig:al}
\end{figure}

\begin{figure}[htb!]
    \centering
        \includegraphics[width=0.7\linewidth]{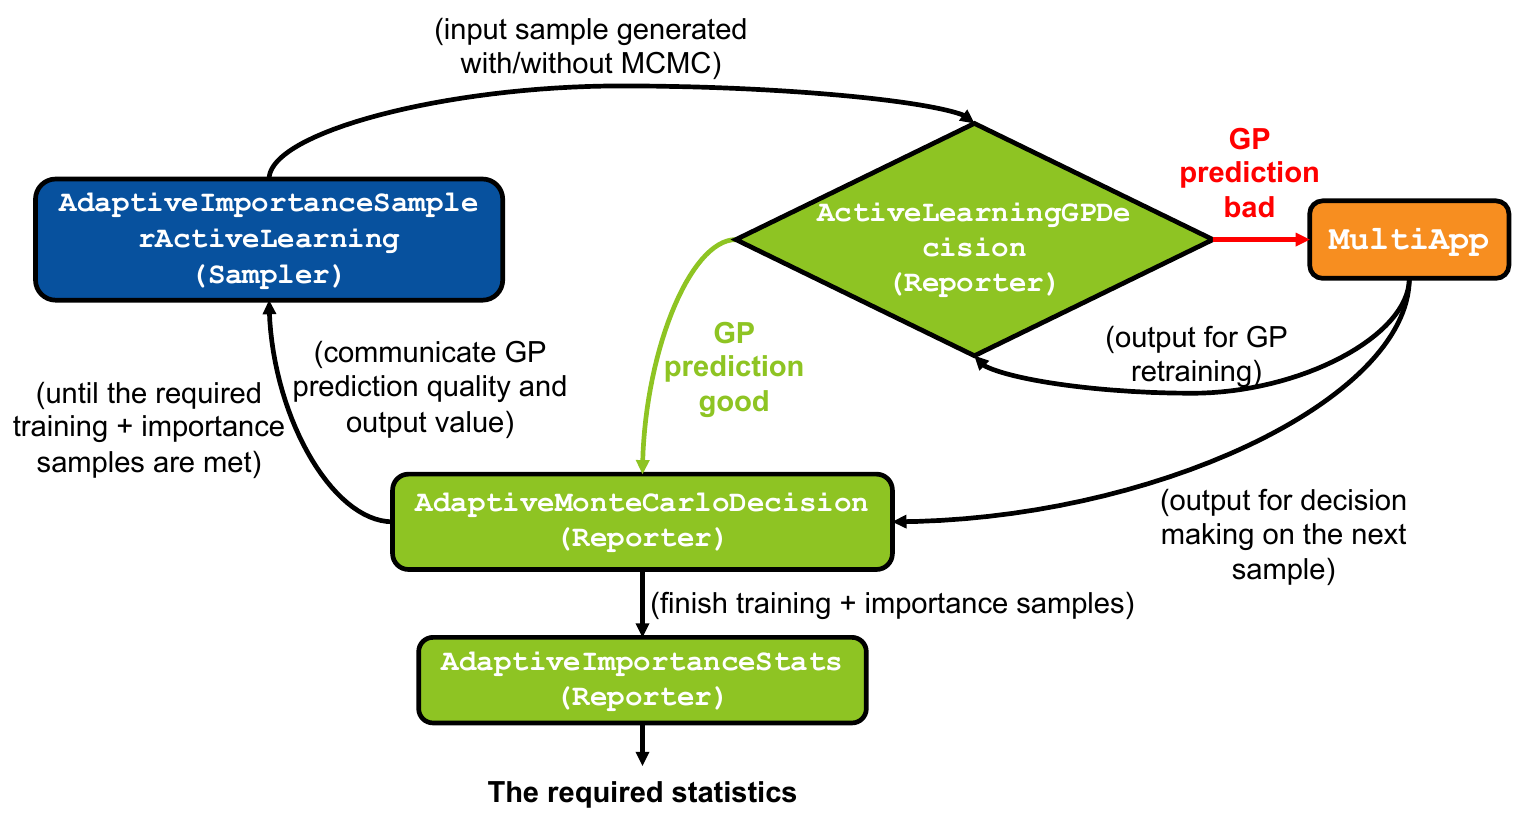}
    \caption{}
    \label{fig:al_ais}
\end{figure}

\begin{figure}[htb!]
    \centering
        \includegraphics[width=0.6\linewidth]{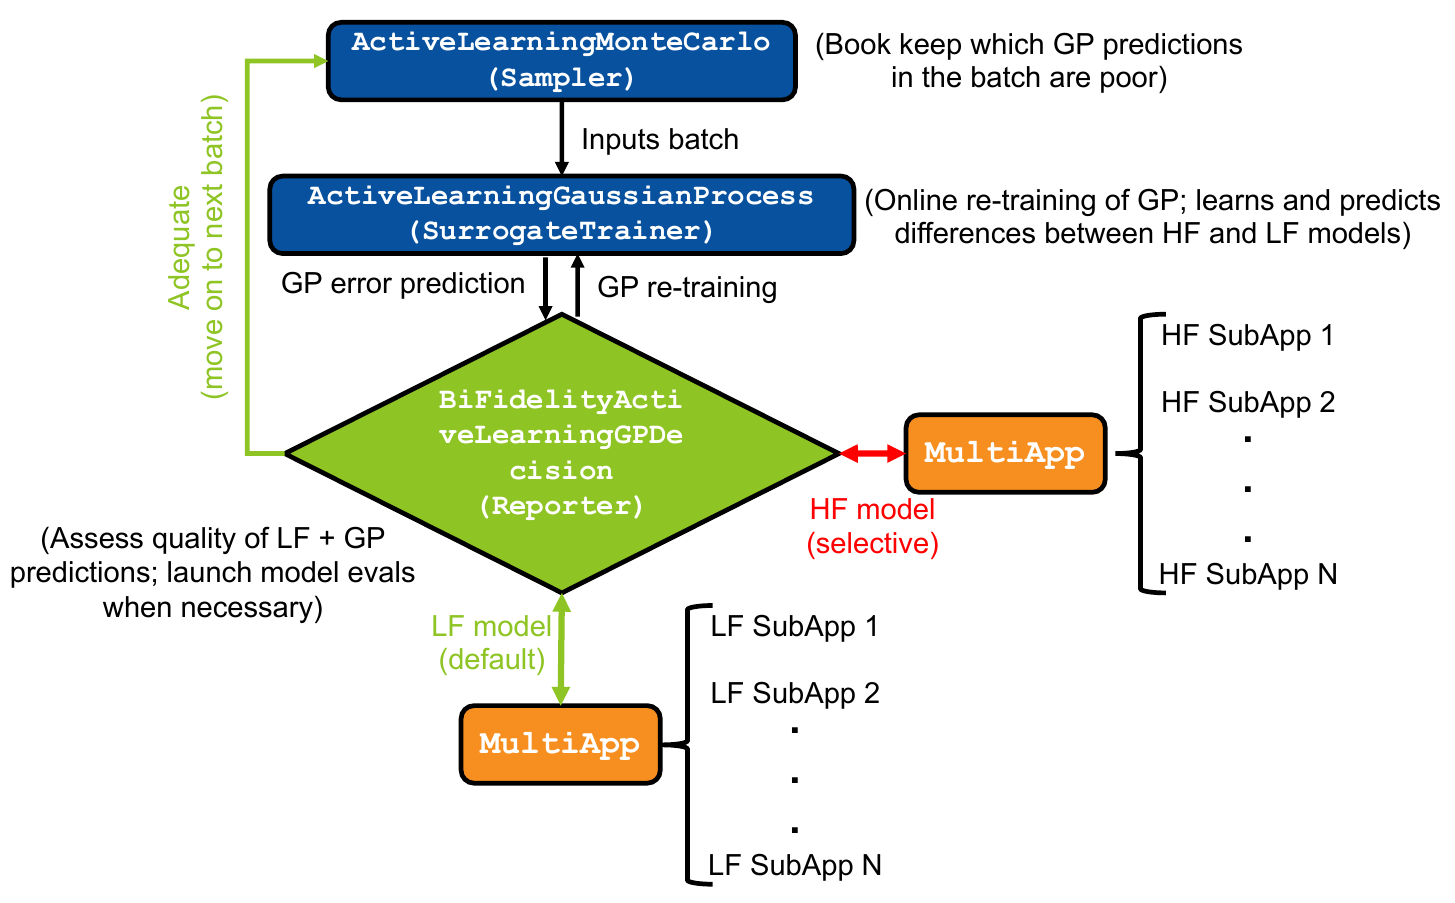}
    \caption{}
    \label{fig:al_bf}
\end{figure}
